# Supplementary material for: A Long Horizon Planning Framework for Manipulating Rigid Pointcloud Objects
Source: arXiv:2011.08177 source file (2020-11-16)
Supplement: Supplementary file 1 [file real_pcd_supplement.tex]

\begin{figure}
    \centering
  \begin{tabular}{c|c}
     \begin{subfigure}{0.31\linewidth}
		\includegraphics[width=1.0\linewidth]{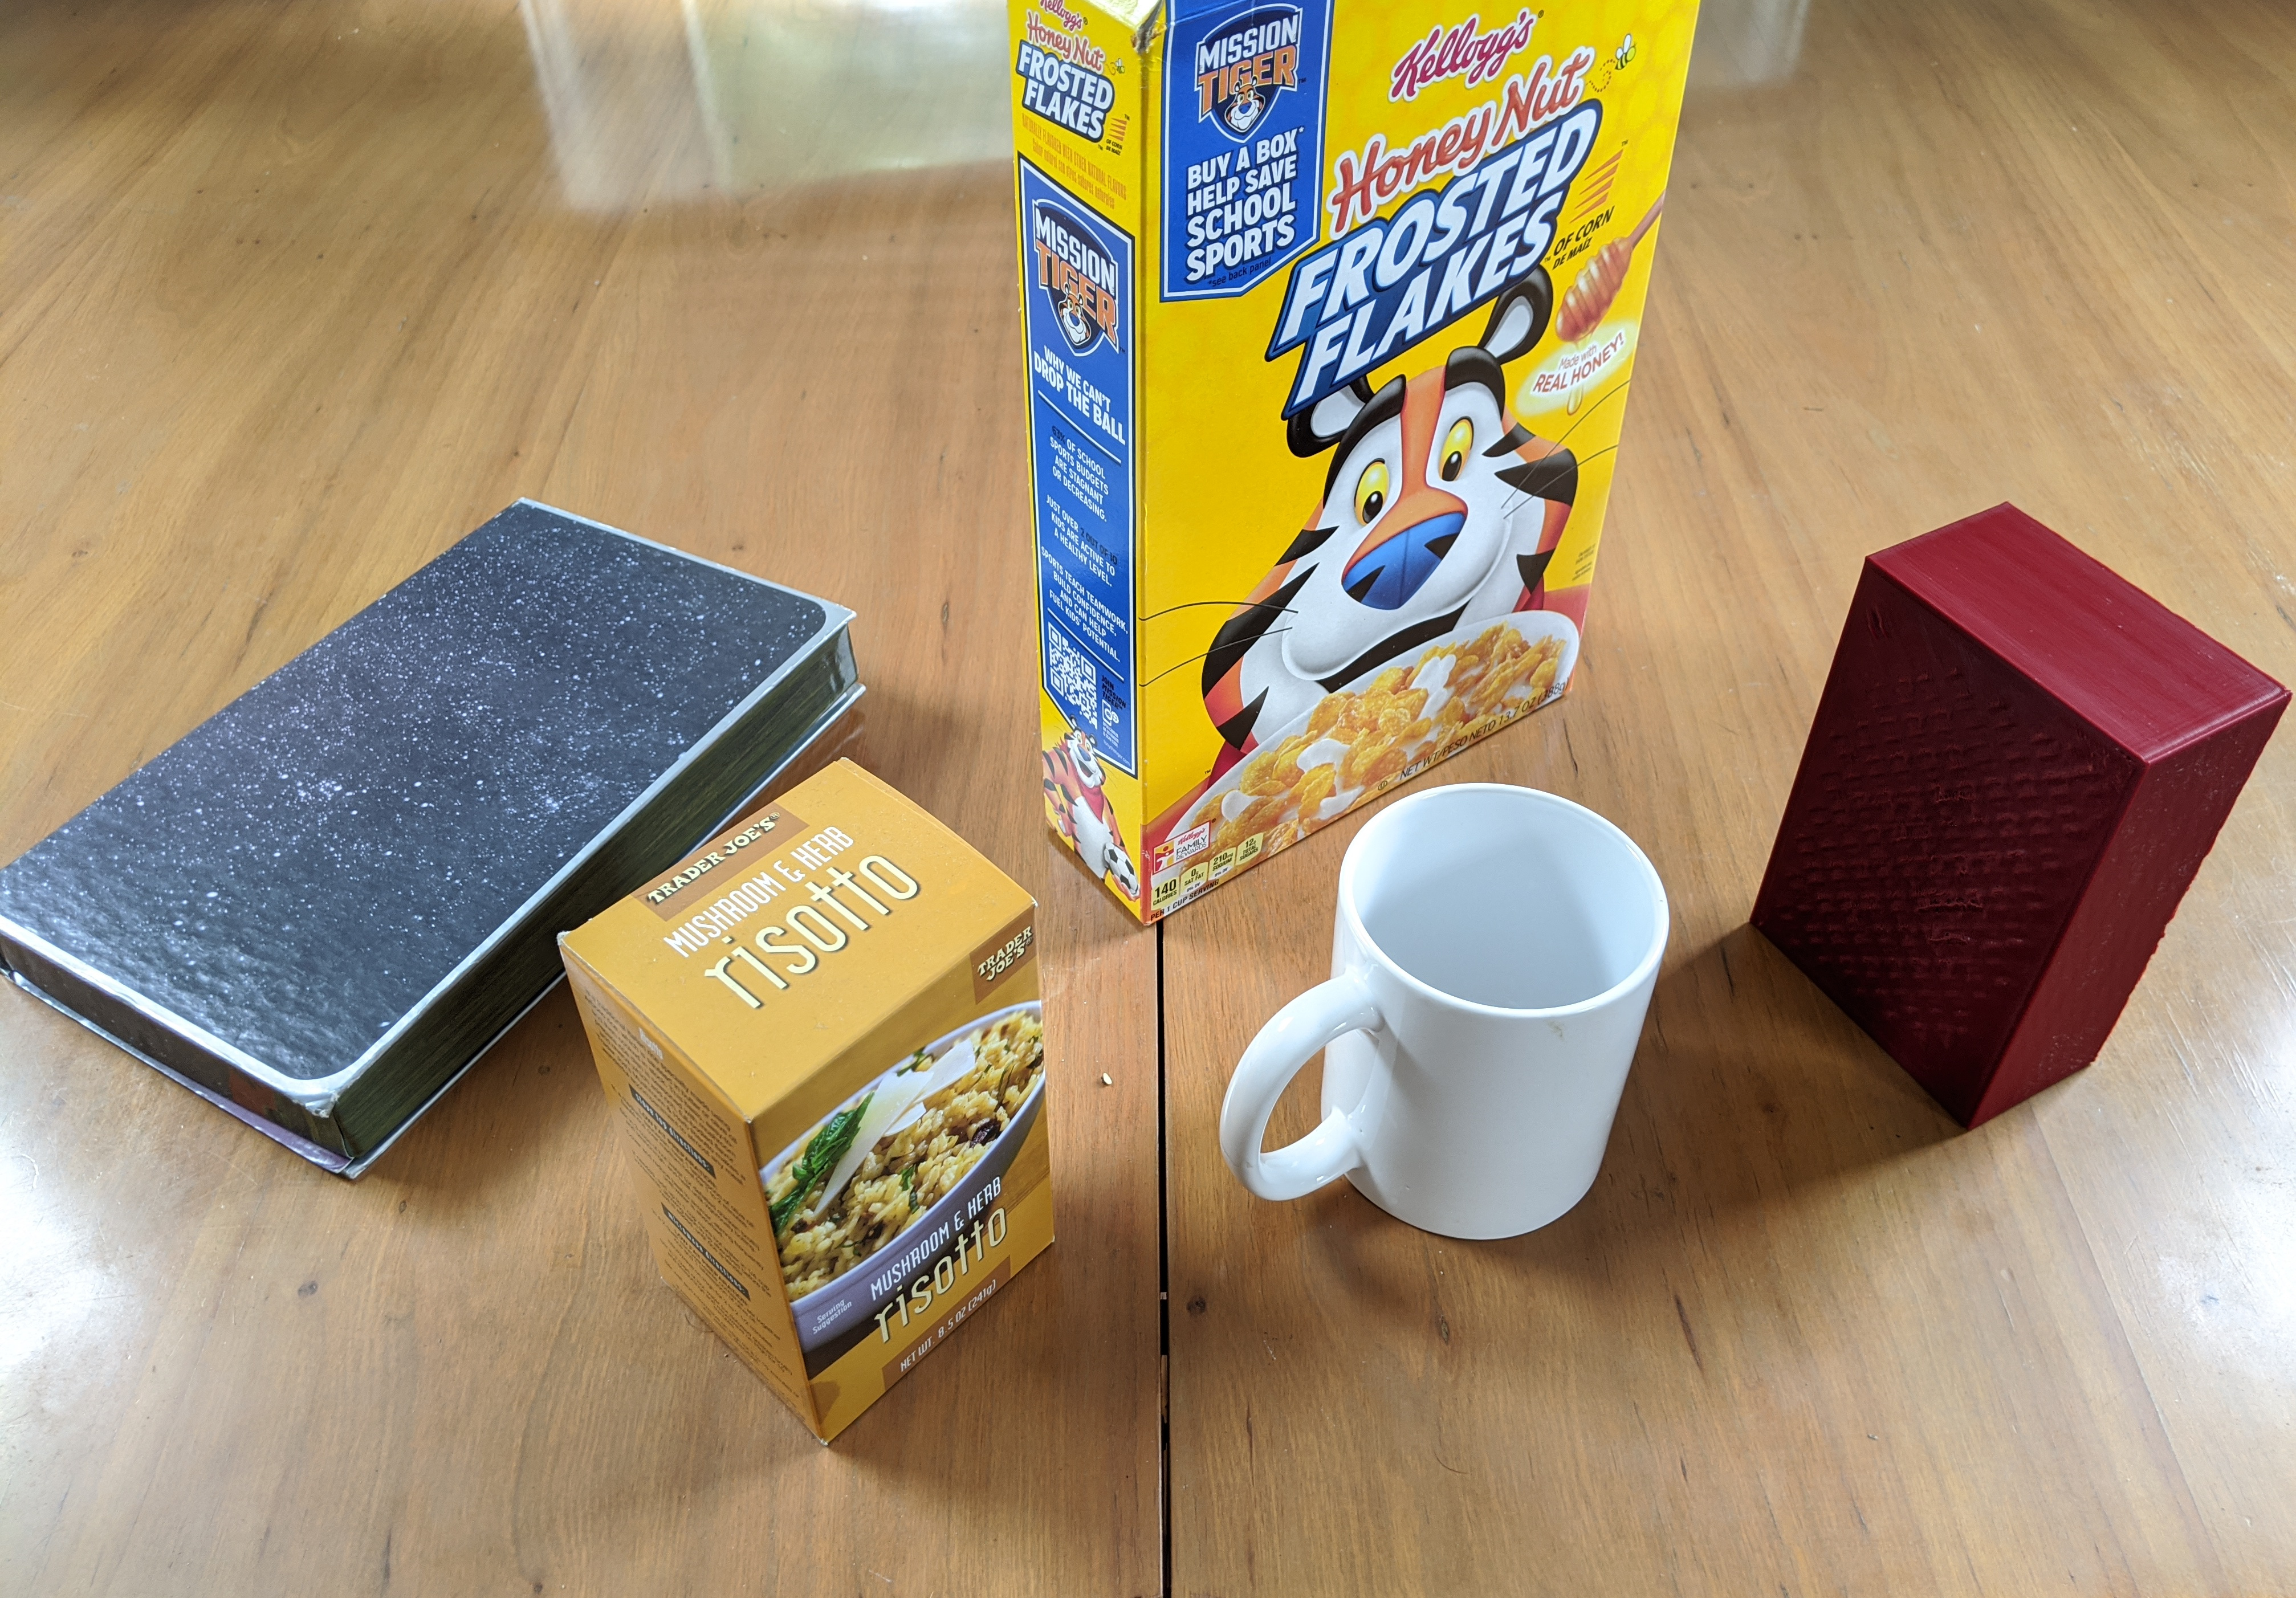}
		\caption{} 
		\label{fig:real-objects}
	\end{subfigure}&
    \begin{subfigure}{0.57\linewidth}
		\includegraphics[width=1.0\linewidth]{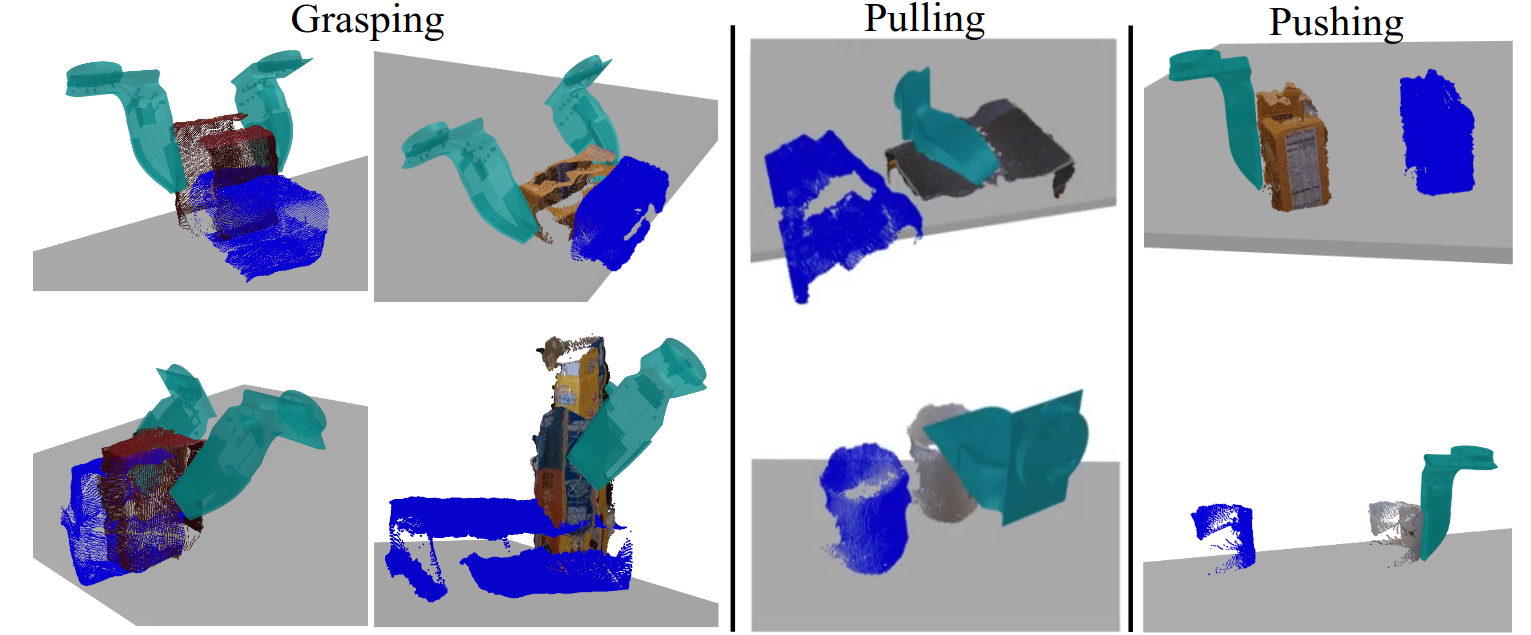}
		\caption{}
		\label{fig:real-object-predictions}
    \end{subfigure}
    \end{tabular}    
    \caption{(a) Objects used for real point-cloud qualitative analysis. (b) Visualization of contact poses (green palms) and subgoals (blue point-clouds) predicted by our learned model for various skills, using real point-cloud objects as input. These results qualitatively support that our framework will generalize to a real-world system.}
    \label{fig: lack-of-experiments}
    \vspace{-20pt}
\end{figure}
